# Supplementary material for: Unmixing Optical Signals from Undersampled Volumetric Measurements by Filtering the Pixel Latent Variables
Source: arXiv:2312.05357 source file (2025-07-11)

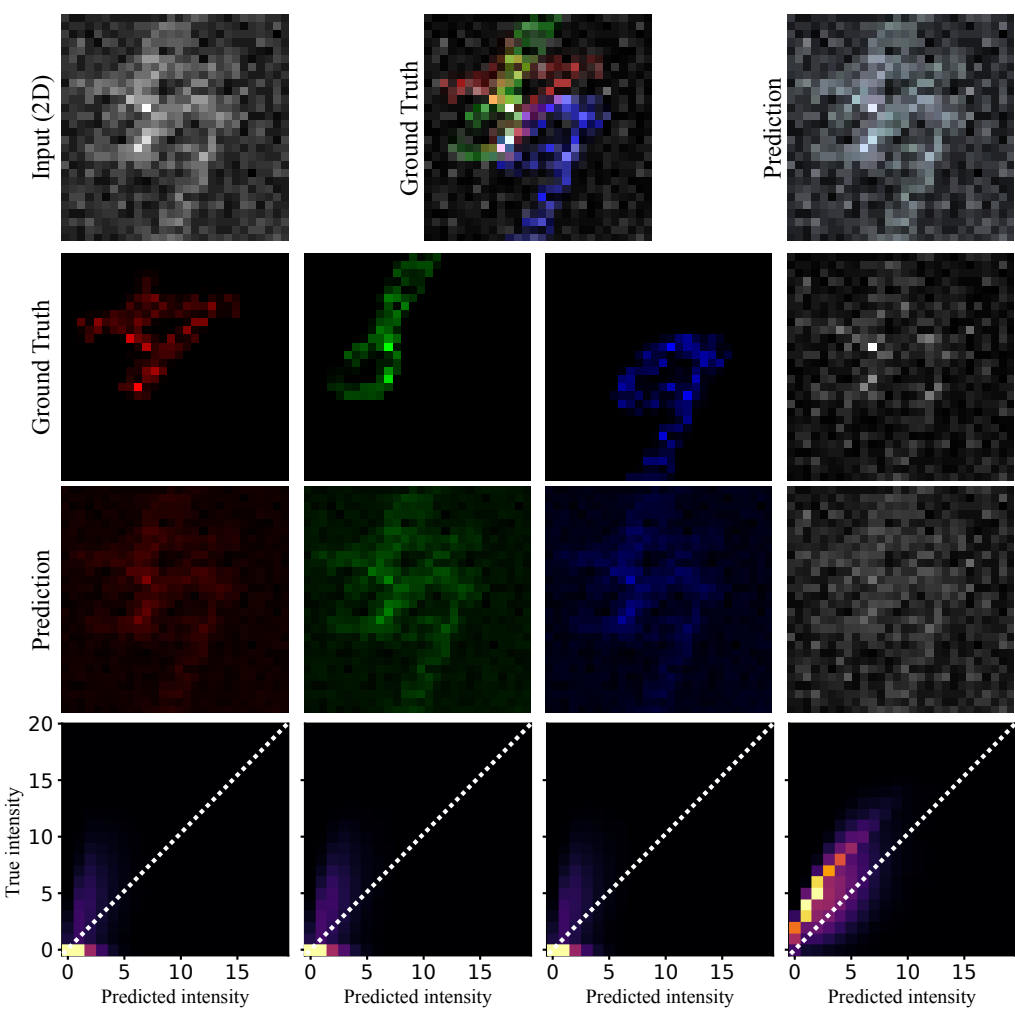

Supplement: Supplementary file 1 [file 2D_MNIST.pdf]
