# Supplementary material for: Unmixing Optical Signals from Undersampled Volumetric Measurements by Filtering the Pixel Latent Variables
Source: arXiv:2312.05357 source file (2025-07-11)

0

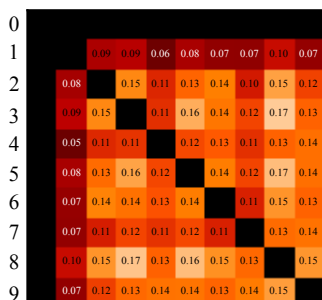

1

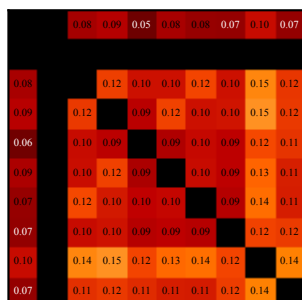

2

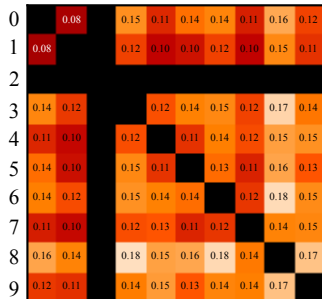

3

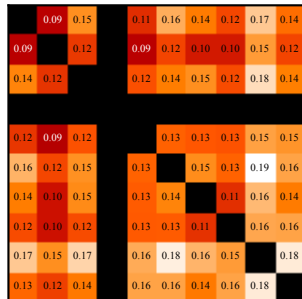

4

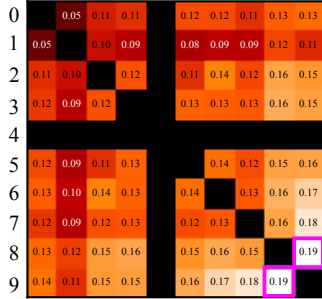

5

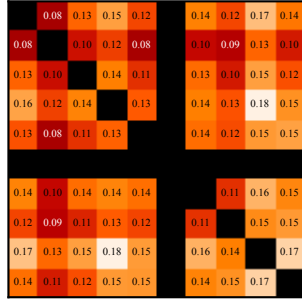

6

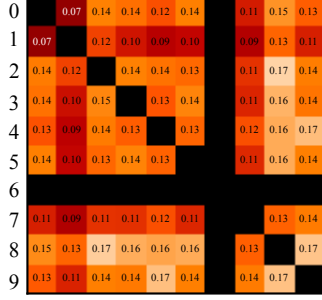

7

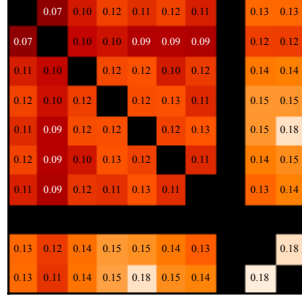

8

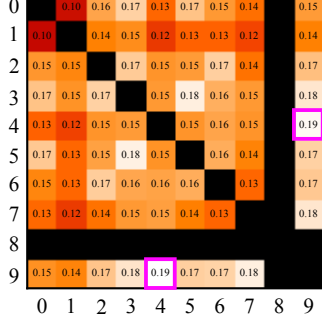

9

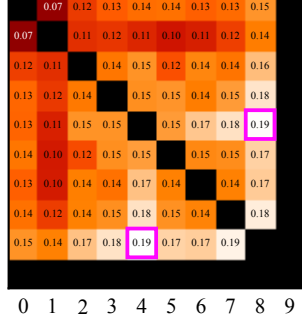

Supplement: Supplementary file 3 [file MNISTOverlap.pdf]
